# Supplementary material for: Foundation for the {\Delta}SCF Approach in Density Functional Theory
Source: arXiv:2403.04604 source file (2024-03-07)
Supplement: Supplementary file 1 [file si_submitted.pdf]

# Supplemental Material: Foundation for the $\Delta SCF$ Approach in Density Functional Theory

Weitao Yang
*Department of Chemistry, Duke University, Durham, North Carolina 27708*[*]

Paul W. Ayers
*Department of Chemistry and Chemical Biology, McMaster University, Hamilton, Ontario L8S 4M1*[†]

## I. PROOF AND NOTES ON LEMMA

**Lemma.** *There is a mapping from the space of excited-state v-representable wavefunctions to their corresponding potentials and excitation levels.*

*Proof.* Recall that a wavefunction, $|\Psi\rangle$, is excited-state $v$-representable only if there exists some Hamiltonian,

$$\hat{H}_w^\lambda = \hat{T} + \lambda V_{ee} + \sum_{i=1}^{N} w(\mathbf{r}_i), \tag{1}$$

for which $|\Psi\rangle$ is an eigenstate. Suppose there were two such Hamiltonians, $H_w^\lambda$ and $H_{w'}^\lambda$, whose local potentials differ by more than a constant. Thus

$$H_w^\lambda |\Psi\rangle = E_{n,w}^\lambda |\Psi\rangle$$
$$H_{w'}^\lambda |\Psi\rangle = E_{n',w'}^\lambda |\Psi\rangle$$

Taking the difference between these two equations,

$$\sum_{i=1}^{N} \left(w(\mathbf{r}_i) - w'(\mathbf{r}_i)\right) |\Psi\rangle = \left(E_{n,w}^\lambda - E_{n',w'}^\lambda\right) |\Psi\rangle \tag{2}$$

To satisfy Eq. (2), $|\Psi\rangle$ must be an eigenstate of $\sum_{i=1}^{N} \left(w(\mathbf{r}_i) - w'(\mathbf{r}_i)\right)$, which is an operator local in physical space. This operator commutes with neither $\hat{H}_w$ nor $\hat{H}_{w'}$, and its eigenfunctions are products of Dirac delta functions, contradicting the initial assumption that $|\Psi\rangle$ is an eigenfunction of these Hamiltonians. Therefore $w(\mathbf{r})$, and hence the Hamiltonian $H_w^\lambda$, are uniquely determined by the excited-state eigenstate $|\Psi\rangle$. The excitation quantum number $n$ can be determined by solving the Schrödinger equation for the Hamiltonian $H_w^\lambda$ and determining which eigenstate corresponds to $\Psi$. □

**Note.** *The proof is the same as in the ground state, and is subject to the same restriction on the space of considered potentials.[1] It is sensible, but not essential, to define an eigenfunction's excitation level as the dimension of the subspace of wavefunctions with lower energy. The mapping from wavefunction to potential and excitation level is invertible if and only if the excited state is nondegenerate.*

This lemma justifies our decision to label wavefunctions, $\Psi_{n,w}^\lambda$, densities, $\rho_{n,w}^\lambda$, and density matrices, $\gamma_{n,w}^\lambda(\mathbf{r},\mathbf{r}')$ with their corresponding potentials and excitation levels.

## II. THE CONVERSE OF THEOREMS 1 AND 2: IS THE STATIONARY POTENTIAL UNIQUE?

In the ground-state potential functional theory, it is asserted that the *only* stationary point of the universal functional, $E_v^\lambda[0,w]$ occurs when $v(\mathbf{r})$ and $w(\mathbf{r})$ differ by at most a constant.[2] The justification for this statement is the

* weitao.yang@duke.edu
† ayers@mcmaster.ca

realization that the linear response function, $\frac{\delta \rho_{0,w}(\mathbf{r})}{\delta w(\mathbf{r}')}$, is negative semidefinite, together with the *assumption* that it has only zero eigenvalue, corresponding to a constant shift in the potential. We are not aware of a proof for the statement that the zero eigenvalue is nondegenerate, though various plausibility arguments can be made.

The current statements of Theorems 1 and 2 are weaker, because we did not make any assumption about how many zero eigenvalues the indefinite excited-state linear response kernel, $\frac{\delta \rho_{n,w}(\mathbf{r}')}{\delta w(\mathbf{r})}$, in Eq. (3) of the main text. In other words, the null space of the linear density response function, defined by all the eigenstates $y(\mathbf{r})$ such that $\int \frac{\delta \rho_{n,w}(\mathbf{r}')}{\delta w(\mathbf{r})} y(\mathbf{r})\, d\mathbf{r} = 0$. Therefore, *the necessary and sufficient condition* for the stationary solutions in Theorem 1 and Theorem 2 is that $v(\mathbf{r}) - w(\mathbf{r}) = y(\mathbf{r})$ for an eigenvector $y(\mathbf{r})$ in the null space of $\frac{\delta \rho_{n,w}(\mathbf{r}')}{\delta w(\mathbf{r})}$, which includes the trivial case $y(\mathbf{r}) = \text{constant}$. We cannot exclude the possibility of non-trivial $y(\mathbf{r})$, but note that the logic is not specific to the excited states, but also affects ground-state potential functional theory.

To our knowledge, nonphysical solutions of the $\Delta$SCF procedure have not been reported.

**Note.** *The converses to Theorems 1 and 2 are equally sound in the ground- and excited-state cases. Specifically, the energy functional $E_v[n, w]$ is stationary if and only if $w(\mathbf{r})$ differs from the physical potential $v(\mathbf{r})$ by a solution to$\int \frac{\delta \rho_{n,w}(\mathbf{r}')}{\delta w(\mathbf{r})} y(\mathbf{r})\, d\mathbf{r} = 0$ , and in most cases we* ***assume*** *that the only solution to these equations is a $y(\mathbf{r}) = $ constant.*

## III. DEGENERATE STATES: EXTENSIONS AND SPECIAL CONSIDERATIONS

### A. The (In)equivalence of Fundamental Descriptors for Noninteracting Systems

We describe the stationary states of the noninteracting system with three equivalent variables,

- the noninteracting potential and excitation level, $w_s(\mathbf{r})$ and $n_s$.
- the $n_s^{\text{th}}$ eigenfunction of the noninteracting Hamiltonian $H^0_{w_s}$, which can be chosen to be a Slater determinant $\Phi[n_s, w_s]$.
- the noninteracting density matrix from the $n_s^{\text{th}}$ eigenstate of the noninteracting Hamiltonian, $\gamma_s[n_s, w_s; \mathbf{r}, \mathbf{r}']$.

It is obvious that $\Phi$ and $\gamma_s$ are determined by the noninteracting state's label and its potential, although for degenerate states the mapping is one-to-many. However, in defining the functionals $E_v[\Phi]$ and $E_v[\gamma_s]$ we use the inverse mapping:

$$E_v\left[\Phi\right] = E_v\left[n_s[\Phi], w_s[\Phi]\right]. \tag{3}$$

Similarly, an excited-state one-electron density matrix, $\gamma_s(\mathbf{r}, \mathbf{r}')$, determines $n_s$ and $w_s$. We thus define a (noninteracting) density-matrix functional,

$$E_v\left[\gamma_s(\mathbf{r}, \mathbf{r}')\right] = E_v\left[n_s[\gamma_s], w_s[\gamma_s]\right]. \tag{4}$$

The inverse mapping $\Phi \to \{n_s, w_s(\mathbf{r})\}$ follows from the Lemma (in the noninteracting limit). For the density matrix, we know three ways to construct the mapping.

#### 1. *First Approach: Invert the Kohn-Sham Equations*

Let $\phi_k(\mathbf{r})$ denote any natural orbital of $\gamma_s$. Then, by inverting the one-electron Schrödinger equation,

$$\left(-\tfrac{1}{2}\nabla^2 + w_s(\mathbf{r})\right)\phi_k(\mathbf{r}) = \epsilon_k \phi_k(\mathbf{r}) \tag{5}$$

one can determine the noninteracting potential, $w_s(\mathbf{r})$. Using the occupation numbers of the natural orbitals, one can identify the excited state to which $\gamma_s$ belongs. For degenerate excited states, the labelling of the degenerate states with $n_s$ is arbitrary, but a suitable label can nonetheless be deduced from $\gamma_s$. This approach exploits the one-electron analogue of the Lemma or, explicitly,

$$w_s(\mathbf{r}) + \text{constant} = \frac{\nabla^2 \phi_k(\mathbf{r})}{2\phi_k(\mathbf{r})} \tag{6}$$

This recalls density-functional approaches where only a small subset of the Kohn-Sham orbitals are used to determine the state of the system.[3–6]

### 2. *Second Approach: Reconstruct a Noninteracting Wavefunction*

Even when $n_s$ denotes a degenerate state, the noninteracting density matrix is easily determined from the eigenfunctions of the noninteracting Hamiltonian $\hat{H}^0_{n_s,w_s} = \hat{H}_s$. When the highest occupied spin-orbital energy is $f$-fold degenerate and the manifold of degenerate orbitals contains $N_f$ electrons, there are $g = \binom{f}{N_f}$ degenerate Slater determinant wavefunctions and the degenerate eigenstates are,

$$|\Psi_s\rangle = \sum_{p=1}^{g} c_p \, |\Phi_p\rangle \tag{7}$$

where

$$1 = \sum_{p=1}^{g} |c_p|^2 \tag{8}$$

The one-electron density matrix has the form,

$$\gamma_s(\mathbf{x}, \mathbf{x}') = \sum_{i=1}^{N-N_f} \phi_i(\mathbf{x})\phi_i^*(\mathbf{x}') + \sum_{i=N-N_f+1}^{N-N_f+f} \sum_{j=N-N_f+1}^{N-N_f+f} \gamma_{ij}\phi_i(\mathbf{x})\phi_j^*(\mathbf{x}') \tag{9}$$

where

$$\gamma_{ij} = \sum_{p=1}^{g}\sum_{q=1}^{g} c_p c_q^* \left\langle \Phi_q \,\middle|\, a_j^\dagger a_i \,\middle|\, \Phi_p \right\rangle \tag{10}$$

Here $a_i^\dagger$ and $a_i$ denote the second-quantized operators for the creation/removal of an electron in a spin-orbital $i$. For simplicity we have used the composite spin+spatial index $\mathbf{x} = \{\mathbf{r}, \sigma\}$ here, so that the occupation numbers are between zero and one instead of between zero and two.

Inverting Eqs. (10) to determine the noninteracting wavefunction $\Psi_s$ is generally impossible: when $2 < N_f < f - 2$ there are more unknown coefficients $\{c_p\}$ than there are density matrix elements $\gamma_{ij}$. Even when this is not true, the mapping from $\gamma_s$ to $\Phi$ is not unique. As a counterexample, consider a case where the only nonzero $c_p$ correspond to $\Phi_p$ which differ by two or more spin-orbitals. The resulting $\gamma_{ij}$ is diagonal and while one may determine $|c_p|^2$, one cannot determine the sign relative signs of the coefficients from $\gamma_{ij}$. However, it is not essential that $\gamma_s$ determines $\Phi$ be unique: one uses Eqs. (10) to select *any one of* the $\Psi_s$ in the degenerate manifold and then uses the Lemma to determine $n_s$ and $w_s(\mathbf{r})$ that correspond to $\Psi_s$, and thus $\gamma_s$.

Thus, for a noninteracting Hamiltonian with a degenerate ground state the mapping from $\{w_s, n_s\}$ to the noninteracting wavefunction $|\Psi_s\rangle$ and density matrix $\gamma_s(\mathbf{x}, \mathbf{x}')$ holds (but is, in general, one-to-many). However, the reverse mapping is unique (up to an arbitrary choice for how one assigns $n_s$ for degenerate states). In addition, the mapping from $\gamma_s$ to the noninteracting wavefunction is one-to-many, but the reverse mapping is unique.

### 3. *Third Approach: Density-Matrix Analogue of the Invertibility Lemma*

The noninteracting density matrix commutes with the one-electron Hamiltonian,

$$0 = \int \left(h_{w_s}(\mathbf{r}, \mathbf{r}')\gamma_s(\mathbf{r}', \mathbf{r}'') - \gamma(\mathbf{r}, \mathbf{r}')h_{w_s}(\mathbf{r}', \mathbf{r}'')\right) d\mathbf{r}' \tag{11}$$

where

$$0 = h_{w_s}(\mathbf{r}, \mathbf{r}') = \delta(\mathbf{r} - \mathbf{r}')\left(-\tfrac{1}{2}\nabla^2_{\mathbf{r}} + w_s(\mathbf{r})\right) \tag{12}$$

Analogous to the proof of the Lemma, we suppose that the noninteracting density matrix also commuted with a different one-electron Hamiltonian. I.e.,

$$0 = \int \left(h_{w_s'}(\mathbf{r}, \mathbf{r}')\gamma_s(\mathbf{r}', \mathbf{r}'') - \gamma(\mathbf{r}, \mathbf{r}')h_{w_s'}(\mathbf{r}', \mathbf{r}'')\right) d\mathbf{r}' \tag{13}$$

Subtracting Eq. (13) from Eq. (11), obtaining

$$0 = \left[(w_s(\mathbf{r}) - w_s'(\mathbf{r})) - (w_s(\mathbf{r}'') - w_s'(\mathbf{r}''))\right]\gamma_s(\mathbf{r}, \mathbf{r}'') \tag{14}$$

This equation is not true unless $w_s(\mathbf{r}) - w_s'(\mathbf{r})$ is independent of position, $\mathbf{r}$. I.e., $w_s(\mathbf{r})$ and $w_s'(\mathbf{r})$ differ by at most a constant.

## B. Theorems 1 and 2 and Their Extension to Degenerate States

Intuitively, Theorems 1 and 2 should hold for degenerate states because one can always make an infinitesimal perturbation of the (non)interacting potential that fully breaks the degeneracy, so that the nondegenerate theorems established in the main text can be used. Nonetheless, it seems useful to show that Theorems 1 and 2 can be applied *directly* to degenerate states.

For degenerate states, there are multiple degenerate eigenstates for a given potential and the linear response function, $\frac{\delta\rho^{\lambda}_{n,w}(\mathbf{r})}{\delta w(\mathbf{r})}$, does not exist because infinitesimal degeneracy-breaking changes in potentials can induce finite changes in the electron density. This changes the proofs of Theorems 1 and 2, but does not change their content. The basic strategy is to first select one of the degenerate interacting wavefunction, $\Psi^{\lambda}_{n,w,v}$, or noninteracting wavefunction, $\Phi_{n_s,w_s,v}$, and use them to define the zeroth-order state. Due to the degeneracy, the functional derivatives $\frac{\delta\rho_{\Psi^{\lambda}_{n,w,v}}(\mathbf{r})}{\delta w(\mathbf{r}')}$ and $\frac{\delta\rho_{\Phi_{n_s,w_s,v}}(\mathbf{r})}{\delta w_s(\mathbf{r}')}$ need not exist, but one can formulate the Gateaux variation, which suffices to prove the theorems.

### 1. *Extension of Theorem 1 to Degenerate States*

Suppose that the $n^{\text{th}}$ state $H^{\lambda}_{w}$ is $g$-fold degenerate. Denote a basis for the degenerate states as $\left\{\Psi^{\lambda}_{p,w}\right\}$. Any degenerate state can be expressed as

$$\Psi^{\lambda}_{n,w}(\{c_p\}) = \sum_{p=1}^{g} c_p \Psi^{\lambda}_{p,w} \tag{15}$$

where $\{c_p\}$ satisfy the normalization condition (8). We generalize the potential-functional for the energy to degenerate states by defining,

$$E^{\lambda}_{v}[n,w] = \min_{\left\{ c_p \,\middle|\, 1=\sum_{p=1}^{g}|c_p|^2 \right\}} \left\langle \Psi^{\lambda}_{n,w}(\{c_p\}) \,\middle|\, H^{\lambda}_{v} \,\middle|\, \Psi^{\lambda}_{n,w}(\{c_p\}) \right\rangle \tag{16}$$

(Just as for ground states, extending our formulation to ensembles is as simple as replacing the minimization over pure states with a minimization of mixed states.[2]) Eq. (16) defines the fundamental energy functional in the potential-functional theory and clearly reduces to the nondegenerate form in the main body of the paper (cf. Eq. (2) therein) when the state is nondegenerate. It is helpful to simplify Eq. (16) by recalling that

$$\hat{H}^{\lambda}_{v} = \hat{H}^{\lambda}_{w} + \sum_{i=1}^{N} \left(v(\mathbf{r}_i) - w(\mathbf{r}_i)\right) \tag{17}$$

Therefore,

$$E^{\lambda}_{v}[n,w] = E^{\lambda}_{n,w} + \min_{\left\{ c_p \,\middle|\, 1=\sum_{p=1}^{g}|c_p|^2 \right\}} \left\langle \Psi^{\lambda}_{n,w}(\{c_p\}) \,\middle|\, \sum_{i=1}^{N} v(\mathbf{r}_i) - w(\mathbf{r}_i) \,\middle|\, \Psi^{\lambda}_{n,w}(\{c_p\}) \right\rangle \tag{18}$$

The minimizing wavefunction in Eq. (16) is a functional of $v(\mathbf{r})$ and we denote it and its corresponding electron density as $\Psi^{\lambda}_{n,w,v}$ and $\rho^{\lambda}_{n,w,v}$, respectively. For most choices of $v(\mathbf{r})$, the minimum in Eq. (16) will be unique. However, when the lowest eigenvalue of the perturbation matrix,

$$V^{\lambda}_{n,w}[v-w]_{pq} = \left\langle \Psi^{\lambda}_{p,w} \,\middle|\, \sum_{i=1}^{N} v(\mathbf{r}_i) - w(\mathbf{r}_i) \,\middle|\, \Psi^{\lambda}_{q,w} \right\rangle \tag{19}$$

is degenerate, the choice of $\{c_p\}$ is not unique.

**Case 1. The minimizing values of $\{c_p\}$ are unique.**

When one varies $w(\mathbf{r})$ the degree of degeneracy is ordinarily reduced. However, *the subspace spanned by the manifold of degenerate states changes only to first order.* Thus, while $\Psi^{\lambda}_{p,w+\delta w} - \Psi^{\lambda}_{p,w}$ is usually $\mathcal{O}(1)$, the change in the value

of Eq. (16) and its minimizing wavefunction remain $\mathcal{O}(||\delta w||)$. Specifically,

$$\begin{aligned} \delta\Psi^{\lambda}_{n,w,v} &= \Psi^{\lambda}_{n,w+\delta w,v} - \Psi^{\lambda}_{n,w,v} \\ &= \sum_{p=1}^{g}\left(\left[\int \frac{\delta c_{p,w,v}}{\delta w(\mathbf{r})}\delta w(\mathbf{r})\, d\mathbf{r}\right]\Psi^{\lambda}_{p,w} + c_{p,w,v}\sum_{\{\, k \,\mid\, E^{\lambda}_{k,w}\neq E^{\lambda}_{p,w}\,\}}\left(\frac{\left\langle \Psi^{\lambda}_{k,w}\,\middle|\,\sum_{i=1}^{N}\delta w(\mathbf{r}_i)\,\middle|\,\Psi^{\lambda}_{p,w}\right\rangle}{E^{\lambda}_{p,w}-E^{\lambda}_{k,w}}\right)\Psi^{\lambda}_{k,w}\right) \end{aligned} \tag{20}$$

where $\{c_{p,w,v}\}$ denotes the coefficients that minimize Eq. (16) and the innermost sum is over the *nondegenerate* eigenstates of the system, in keeping with ordinary degenerate perturbation theory. $\frac{\delta c_{p,w,v}}{\delta w(\mathbf{r})}$ exists because the minimum is unique. The variation in the potential functional is then:

$$\begin{aligned} E^{\lambda}_{v}[n,w+\delta w] - E^{\lambda}_{v}[n,w] &= \left\langle \Psi^{\lambda}_{n,w,v}+\delta\Psi^{\lambda}_{n,w,v}\,\middle|\,\hat{H}^{\lambda}_{v}\,\middle|\,\Psi^{\lambda}_{n,w,v}+\delta\Psi^{\lambda}_{n,w,v}\right\rangle - \left\langle \Psi^{\lambda}_{n,w,v}\,\middle|\,\hat{H}^{\lambda}_{v}\,\middle|\,\Psi^{\lambda}_{n,w,v}\right\rangle \\ &= \left\langle \delta\Psi^{\lambda}_{n,w,v}\,\middle|\,\hat{H}^{\lambda}_{v}\,\middle|\,\Psi^{\lambda}_{n,w,v}\right\rangle + \left\langle \Psi^{\lambda}_{n,w,v}\,\middle|\,\hat{H}^{\lambda}_{v}\,\middle|\,\delta\Psi^{\lambda}_{n,w,v}\right\rangle \\ &= \left\langle \delta\Psi^{\lambda}_{n,w,v}\,\middle|\,\hat{H}^{\lambda}_{w}\,\middle|\,\Psi^{\lambda}_{n,w,v}\right\rangle + \left\langle \Psi^{\lambda}_{n,w,v}\,\middle|\,\hat{H}^{\lambda}_{w}\,\middle|\,\delta\Psi^{\lambda}_{n,w,v}\right\rangle \\ &\quad + \left\langle \delta\Psi^{\lambda}_{n,w,v}\,\middle|\,\sum_{i=1}^{N} v(\mathbf{r}_i)-w(\mathbf{r}_i)\,\middle|\,\Psi^{\lambda}_{n,w,v}\right\rangle + \left\langle \Psi^{\lambda}_{n,w,v}\,\middle|\,\sum_{i=1}^{N} v(\mathbf{r}_i)-w(\mathbf{r}_i)\,\middle|\,\delta\Psi^{\lambda}_{n,w,v}\right\rangle \\ &= \int (v(\mathbf{r})-w(\mathbf{r}))\delta\rho^{\lambda}_{n,w,v}(\mathbf{r}))\, d\mathbf{r} \end{aligned} \tag{21}$$

In the next to last equality we used the fact $\Psi^{\lambda}_{n,w,v}$ is an eigenfunction of $\hat{H}^{\lambda}_{w}$ and the fact that an eigenfunction is orthogonal to its perturbation, $\left\langle \delta\Psi^{\lambda}_{n,w,v}\,\middle|\,\Psi^{\lambda}_{n,w,v}\right\rangle = 0$ (cf. Eq. (22)). Because $\delta\rho^{\lambda}_{n,w,v}(\mathbf{r})$ is normalized to zero, Eq. (21) is zero when $v(\mathbf{r})-w(\mathbf{r})$ is a constant.

**Case 2. The minimizing values of $\{c_p\}$ are not unique.**

When there is not a unique minimizing function in Eq. (16), most choices of $\delta w(\mathbf{r})$ will fully remove the degeneracy, giving different choices for the minimizing coefficients for different $\delta w(\mathbf{r})$. Eq. (22) is no longer valid because $\frac{\delta c_{p,w,v}}{\delta w(\mathbf{r})}$ does not exist. Since $c_{p,w+\delta w,v}$ depends on the specific choice of $\delta w(\mathbf{r})$, the functional derivative $\frac{\delta c_{p,w,v}}{\delta w(\mathbf{r})}$ does not exist and only the Gateaux variation exists. To determine the optimal coefficients, we insert $w+\delta w$ in Eq. (19) and find the lowest eigenvalue of $V^{\lambda}_{n,w}[v-w-\delta w]_{pq}$ and its associated eigenvector. We then use $V^{\lambda}_{n,w}[v-w-\delta w]_{pq}$ as the unperturbed system and $V^{\lambda}_{n,w}[v-w]_{pq}$ as the perturbed system, so that we can determine the change in the lowest eigenvalue and its eigenvector associated with removal of the potential $\delta w(\mathbf{r})$. This defines for the optimal coefficients $c_{p,w,v}[\delta w]$ and their Gateaux variation, $dc_{p,w,v}[\delta w]$. The Gateaux variation only vanishes if all the eigenvalues of the unmodified perturbation matrix, $V^{\lambda}_{n,w}[v-w]_{pq}$, are the same or if the specific variation $\delta w(\mathbf{r})$ does not couple the eigenspace of the lowest eigenvalues of $V^{\lambda}_{n,w}[v-w]_{pq}$ to its other eigenvectors. When the lowest eigenvalue of $V^{\lambda}_{n,w}[v-w-\delta w]_{pq}$ is degenerate, the Gateaux variation is not unique, but the following analysis does not depend on how one selects among the infinite number of acceptable choices.

The wavefunction is no longer differentiable with respect to $\delta w(\mathbf{r})$, but its Gateaux variation is:

$$\begin{aligned} \delta\Psi^{\lambda}_{n,w,v}[\delta w] &= \Psi^{\lambda}_{n,w+\delta w,v} - \Psi^{\lambda}_{n,w,v} \\ &= \sum_{p=1}^{g}\left( dc_{p,w,v}[\delta w]\Psi^{\lambda}_{p,w} + c_{p,w,v}[\delta w]\sum_{\{\, k \,\mid\, E^{\lambda}_{k,w}\neq E^{\lambda}_{p,w}\,\}}\left(\frac{\left\langle \Psi^{\lambda}_{k,w}\,\middle|\,\sum_{i=1}^{N}\delta w(\mathbf{r}_i)\,\middle|\,\Psi^{\lambda}_{p,w}\right\rangle}{E^{\lambda}_{p,w}-E^{\lambda}_{k,w}}\right)\Psi^{\lambda}_{k,w}\right) \end{aligned} \tag{22}$$

Using this notation, the derivation (21) holds exactly as before, giving the final result

$$E^{\lambda}_{v}[n,w+\delta w] - E^{\lambda}_{v}[n,w] = \int (v(\mathbf{r})-w(\mathbf{r}))\,\delta\rho^{\lambda}_{n,w,v}[\delta w;\mathbf{r}]\, d\mathbf{r} \tag{23}$$

Eq. (23) is zero when $v(\mathbf{r})-w(\mathbf{r})$ is a constant. The resulting general statement of Theorem 1 is:

**Theorem 1.** *The Gateaux variation of $E^{\lambda}_{v}[n,w]$, as defined in Eq. (16), with respect to the trial potential, $w(\mathbf{r})$, is zero when $w(\mathbf{r})$ and the physical potential, $v(\mathbf{r})$, differ by at most a constant.*

For nondegenerate states, the Gateaux variation can be replaced by the functional derivative, establishing the equivalence to Theorem 1 in the main text.

### 2. Extension of Theorem 2 to Degenerate States

While $E_v[n_s, w_s]$ has the same value as $E_v^1[n, w]$, the variation is now with respect to the noninteracting potential. When the noninteracting state, $\{n_s, w_s(\mathbf{r})\}$, is degenerate, there are many densities associated with it and, except when the degeneracy is driven by a fundamental physical symmetry of the system, each of these densities may correspond to a different physical state. We need to define the functionals $n[n_s, w_s]$ and $w[n_s, w_s]$ so that we can assign $E_v[n_s, w_s] = E_v^1\,[n[n_s, w_s], w[n_s, w_s]]$. This requires specifying one of the electron densities associated with the noninteracting system, so that we can identify an interacting system, with $\{n, w(\mathbf{r})\}$ with the same electron density.

Analogous to the ground-state potential functional theory,[2] we select the degenerate noninteracting wavefunction that gives the lowest energy for the physical system. Specifically, let

$$\Phi_{n_s,w_s}(\{c_p\}) = \sum_{p=1}^{g} c_p \Phi_{p,w_s} \tag{24}$$

where $\{c_p\}$ satisfy the normalization condition (8). Then we define

$$E_v\left[\Phi[n_s, w_s, v]\right] = \min_{\left\{ c_p \;\middle|\; 1=\sum_{p=1}^{g} |c_p|^2 \right\}} \left\langle \Phi_{n_s,w_s}(\{c_p\}) \,\middle|\, H_v^1 \,\middle|\, \Phi_{n_s,w_s}(\{c_p\}) \right\rangle \tag{25}$$

**Case 1. The minimizing values of $\{c_p\}$ are unique.** In the simplest case, there is a unique minimum in Eq. (25), corresponding to the noninteracting wavefunction, $\Phi_{n_s,w_s,v}$, density matrix $\gamma_{n_s,w_s,v}(\mathbf{r}, \mathbf{r}')$, and density $\rho_{n_s,w_s,v}(\mathbf{r})$. According to the excited-state Kohn-Sham assumption, there is a stationary state of an interacting system with the same electron density. Labelling this stationary state with $\{n, w(\mathbf{r})\}$, The potential function is thus defined as $E_v^1[n[n_s, w_s], w[n_s, w_s]]$ As the degeneracy was fully broken, small variations in the noninteracting potential, $\delta w_s(\mathbf{r})$ correspond to small changes in the minimizing noninteracting wavefunction its associated electron density. We *assume* that these small $\mathcal{O}(||\delta w_s||)$ changes in the electron density correspond to $\mathcal{O}(||\delta w_s||)$ or smaller changes in the interacting potential.

With this assumption, Theorem 1 implies Theorem 2. Explicitly, assuming that $w(\mathbf{r}) + \delta w(\mathbf{r})$ is the perturbed interacting external potential corresponding to perturbed noninteracting potential $w_s(\mathbf{r}) + \delta w_s(\mathbf{r})$

$$\begin{aligned}
E_v[n_s, w_s + \delta w_s] - E_v[n_s, w_s] &= E_v^1\left[n[n_s, w_s + \delta w_s] - E_v^1[n[n_s, w_s], [n_s, w_s]\right] \\
&= E_v^1[n, w + \delta w] - E_v^1[n, w] \\
&= \int (v(\mathbf{r}) - w(\mathbf{r}))(\rho_{n_s,w_s+\delta w_s,v}(\mathbf{r}) - \rho_{n_s,w_s,v}(\mathbf{r}))\, d\mathbf{r}
\end{aligned} \tag{26}$$

**Case 2. The minimizing values of $\{c_p\}$ are not unique.** When there is not a unique minimum in Eq. (25), only the Gateaux variation exists. (This is especially likely to occur when the degeneracy arises from a symmetry of the physical system.) In this case, the density depends on the variation of $w_s(\mathbf{r})$ being considered, $\rho_{n_s,w_s,v}[\delta w_s; \mathbf{r}]$. As with Eq. (23), only the Gateaux differential exists, and is given by the expression

$$\begin{aligned}
E_v[n_s, w_s + \delta w_s] - E_v[n_s, w_s] &= E_v^1\left[n[n_s, w_s + \delta w_s] - E_v^1[n[n_s, w_s], [n_s, w_s]\right] \\
&= \int (v(\mathbf{r}) - w(\mathbf{r}))\, \delta\rho^{\lambda}_{n_s,w_s,v}[\delta w_s; \mathbf{r}]\, d\mathbf{r}
\end{aligned} \tag{27}$$

**Note.** *The proof of theorem 2 relies on the assumption that the map from the noninteracting potential to the interacting potential is continuous and differentiable. This assumption is not specific to the degenerate case of the excited-state potential functional theory, but is implicit in the ground-state and the nondegenerate excited-state theories too. Recall that the dielectric function, $\epsilon(\mathbf{r}, \mathbf{r}')$ provides the map from variations in the noninteracting potential to variations in the interacting potential,*

$$\delta w(\mathbf{r}) = \int \epsilon(\mathbf{r}, \mathbf{r}') \delta w_s(\mathbf{r}')\, d\mathbf{r}' \tag{28}$$

*The essential assumption is that the dielectric function is bounded: ergo, infinitesimal changes in $\delta w_s(\mathbf{r})$ map to $\mathcal{O}(||\delta w_s||)$ changes in the interacting potential.*

Theorem 2 indicates that every stationary point of the potential functional $E_v^1[n_s, w_s]$ corresponds to a stationary state of a physical system. The converse need not be true: because the minimization in Eq. (25) selects just one of the noninteracting wavefunctions, $\Phi_{n_s,w_s,v}$, physical systems corresponding to the other degenerate noninteracting states may be inaccessible. This problem can be alleviated when one adopts the orbital-functional, $E_v^1[\Phi]$ or the density-matrix functional $E_v[\gamma_s]$. In particular, one does not need to use Eq. (25): *any* systematic way of specifying the noninteracting wavefunction will suffice for the purposes of the theorem 2. One can thus exploit the one-to-many nature of the $\{n_s, w_s(\mathbf{r})\} \to \Phi_{n_s,w_s}$ mapping discussed in section III A to ensure that all the physical stationary states associated with the degenerate $n_s^{\text{th}}$ stationary-state densities of the noninteracting potential $w_s(\mathbf{r})$ are accessible.

## IV. ADIABATIC CONNECTION

The excited-state Kohn-Sham assumption is that for any physical excited state, described by the excitation level $n$ and external potential $w(\mathbf{r})$, there also exists a noninteracting excited state described by the excitation level $n_s$ and the external potential $w_s(\mathbf{r})$. *Any* pathway connecting these two states can be used to construct a functional. These pathways are defined by a parameterized curve of external potentials, $w^\lambda(\mathbf{r})$, that satisfy the obvious boundary conditions,

$$\begin{aligned} w^1(\mathbf{r}) &= w(\mathbf{r}) \\ w^0(\mathbf{r}) &= w_s(\mathbf{r}) \end{aligned} \tag{29}$$

In the context of potential functional theory, it is especially appealing to use the adiabatic connection based on the linear interpolation of potentials,[7])

$$w^\lambda(\mathbf{r}) = (1-\lambda)w_s(\mathbf{r}) + \lambda w(\mathbf{r}). \tag{30}$$

However, the constant-density adiabatic connection,[8, 9] where $n^\lambda$ and $w^\lambda(\mathbf{r})$ are chosen so that the specified excited state density is preserved all along the adiabatic connection pathway, $\rho_{n,w}(\mathbf{r}) = \langle \Psi^\lambda_{n^\lambda,w^\lambda} | \hat{\rho}(\mathbf{r}) | \Psi^\lambda_{n^\lambda,w^\lambda} \rangle$ gives simpler working equations for the exchange-correlation functional.

The derivation of the adiabatic connection formula is exactly the same as for ground states, but we repeat the analysis here to facilitate later discussion.[8, 10, 11] Specifically, from first-order perturbation theory,

$$\begin{aligned} \frac{dE^\lambda_{n^\lambda,w^\lambda}}{d\lambda} &= \frac{d\left\langle \Psi^\lambda_{n^\lambda,w^\lambda} \middle| \hat{T} + \lambda V_{ee} + \sum_{i=1}^N w^\lambda(\mathbf{r}_i) \middle| \Psi^\lambda_{n^\lambda,w^\lambda} \right\rangle}{d\lambda} \\ &= \left\langle \Psi^\lambda_{n^\lambda,w^\lambda} \middle| V_{ee} + \sum_{i=1}^N \frac{dw^\lambda(\mathbf{r}_i)}{d\lambda} \middle| \Psi^\lambda_{n^\lambda,w^\lambda} \right\rangle \\ &= \left\langle \Psi^\lambda_{n^\lambda,w^\lambda} \middle| V_{ee} \middle| \Psi^\lambda_{n^\lambda,w^\lambda} \right\rangle \\ &\quad + \int \rho_{n^\lambda,w^\lambda}(\mathbf{r}) \frac{dw^\lambda(\mathbf{r})}{d\lambda}\, d\mathbf{r} \end{aligned}$$

Integrating this expression over the adiabatic connection pathway, one obtains

$$\begin{aligned} E^1_{n,w} - E^0_{n_s,w_s} &= \int_0^1 \frac{dE^\lambda_{n^\lambda,w^\lambda}}{d\lambda}\, d\lambda \\ &= \int_0^1 \left\langle \Psi^\lambda_{n^\lambda,w^\lambda} \middle| V_{ee} \middle| \Psi^\lambda_{n^\lambda,w^\lambda} \right\rangle d\lambda \\ &\quad + \int_0^1 \int \rho_{n^\lambda,w^\lambda}(\mathbf{r}) \frac{dw^\lambda(\mathbf{r})}{d\lambda}\, d\mathbf{r}\, d\lambda \end{aligned} \tag{31}$$

The last term can be simplified by defining

$$\Delta^\lambda(\mathbf{r}) = \rho_{n^\lambda,w^\lambda}(\mathbf{r}) - \rho_{n,w}(\mathbf{r}). \tag{32}$$

Then

$$\int_0^1 \rho_{n^\lambda,w^\lambda}(\mathbf{r})\frac{dw^\lambda(\mathbf{r})}{d\lambda}\,d\lambda = \int_0^1 \rho_{n,w}(\mathbf{r})\frac{dw^\lambda(\mathbf{r})}{d\lambda}\,d\lambda + \int_0^1 \Delta^\lambda(\mathbf{r})\frac{dw^\lambda(\mathbf{r})}{d\lambda}\,d\lambda$$
$$= \rho_{n,w}(\mathbf{r})\int_0^1 \frac{dw^\lambda(\mathbf{r})}{d\lambda}\,d\lambda + \int_0^1 \Delta^\lambda(\mathbf{r})\frac{dw^\lambda(\mathbf{r})}{d\lambda}\,d\lambda \tag{33}$$
$$= \rho_{n,w}(\mathbf{r})\left(w(\mathbf{r}) - w_s(\mathbf{r})\right) + \int_0^1 \Delta^\lambda(\mathbf{r})\frac{dw^\lambda(\mathbf{r})}{d\lambda}\,d\lambda$$

The second term vanishes only in the constant-density adiabatic connection. Recall the standard expressions for the energies of the interacting and noninteracting systems,

$$E^1_{n,w}[\Phi] = T_s[\Phi] + J[\rho] + E_{xc}[\Phi] + \int \rho_{n,w}(\mathbf{r})w(\mathbf{r})\,d\mathbf{r}$$
$$E^0_{n_s,w_s}[\Phi] = T_s[\Phi] + \int \rho_{n,w}(\mathbf{r})w_s(\mathbf{r})\,d\mathbf{r} \tag{34}$$

Inserting these expressions into Eq. (31) and simplifying,

$$J[\rho] + E_{xc}[\Phi] = \int_0^1 \left\langle \Psi^\lambda_{n^\lambda,w^\lambda} \middle| V_{ee} \middle| \Psi^\lambda_{n^\lambda,w^\lambda} \right\rangle d\lambda + \int\int_0^1 \Delta^\lambda(\mathbf{r})\frac{dw^\lambda(\mathbf{r})}{d\lambda}\,d\lambda d\mathbf{r} \tag{35}$$

where the last line vanishes for the constant-density adiabatic connection, but not in general.

Recall that the two-electron distribution function can be expressed in terms of the exchange-correlation charge,

$$\rho_2^\lambda(\mathbf{r},\mathbf{r}') = \left\langle \Psi^\lambda_{n^\lambda,w^\lambda} \middle| \sum_{i=1}^N \sum_{j=1}^N \delta(\mathbf{r}_i - \mathbf{r})\delta(\mathbf{r}_j - \mathbf{r}') \middle| \Psi^\lambda_{n^\lambda,w^\lambda} \right\rangle = \rho^\lambda(\mathbf{r})\rho^\lambda(\mathbf{r}') + \rho^\lambda(\mathbf{r})\rho^\lambda_{xc}(\mathbf{r},\mathbf{r}') \tag{36}$$

This gives an explicit expression for the exchange-correlation energy,

$$E_{xc}[\Phi] = \iint \overline{\frac{\rho^\lambda(\mathbf{r})\rho^\lambda(\mathbf{r}')}{|\mathbf{r}-\mathbf{r}'|}}\,d\mathbf{r}d\mathbf{r}' - J[\rho_{n,w}] + \iint \overline{\frac{\rho^\lambda(\mathbf{r})\rho^\lambda_{xc}(\mathbf{r},\mathbf{r}')}{|\mathbf{r}-\mathbf{r}'|}}\,d\mathbf{r}d\mathbf{r}' + \int \overline{\Delta^\lambda(\mathbf{r})\frac{dw^\lambda(\mathbf{r})}{d\lambda}}\,d\mathbf{r} \tag{37}$$

which, for the constant-density adiabatic connection, simplifies to

$$E_{xc}[\Phi] = \iint \frac{\rho_{n,w}(\mathbf{r})\overline{\rho^\lambda_{xc}(\mathbf{r},\mathbf{r}')}}{|\mathbf{r}-\mathbf{r}'|}\,d\mathbf{r}d\mathbf{r}' \tag{38}$$

Here we have introduced the following notation for averaging a function across the adiabatic connection,

$$\overline{f^\lambda(\mathbf{r})} = \int_0^1 f^\lambda(\mathbf{r})\,d\lambda \tag{39}$$

Note that the exchange-correlation functionals thus defined are exactly the same for excited- and ground-states, with working expressions identical to the traditional expressions used in Kohn-Sham density-functional theory.

When $n_s \neq n$, the process of moving along the adiabatic connection is more complicated, though the previous formulae all hold. The main issue is selecting the correct degenerate-state wavefunction, $\Psi^\lambda_{n^\lambda,w^\lambda}$. In the constant-density adiabatic connection, the choice should ordinarily be clear (see the detailed discussion by Görling[9]), but there is no guarantee that the constant-density adiabatic connection exists. For other adiabatic connection pathways, it is

convenient to try to minimize the deviation of the electron density from the target value (i.e., make $\Delta^{\lambda}(\mathbf{r})$ small), but this is not essential. For example, whenever one encounters degeneracy, one could successively increment $n^{\lambda}$ so that it approaches the target value, $n$, for the interacting limit as quickly as possible, and then leave $n^{\lambda}$ fixed thereafter. Different methods will give different *expressions* for the functional, but the stationary points of all of the expressions give the *exact* ground-and-excited-state energies and densities.

As alluded to by Harris and Görling,[9, 10] establishing the existence of the constant-density adiabatic connection requires an analysis of the linear response function. To explain this more explicitly, we define the Hamiltonian

$$\hat{H}^{\mu}_{w^{\lambda}} = \hat{T} + \mu V_{ee} + \sum_{i=1}^{N} w^{\lambda}(\mathbf{r}_i), \tag{40}$$

and denote its eigenfunctions and their associated electron densities as $\Psi^{\mu}_{n^{\lambda},w^{\lambda}}$ and $\rho^{\mu}_{n^{\lambda},w^{\lambda}}(\mathbf{r})$, respectively.

Suppose that at some point on the adiabatic connection pathway, $\lambda_0$, the constant-density condition is satisfied

$$\rho^{\lambda_0}_{n^{\lambda_0},w^{\lambda_0}}(\mathbf{r}) = \rho_{n,w}(\mathbf{r}) = \rho_{n_s,w_s}(\mathbf{r}) \tag{41}$$

Changing the strength of the electron-electron repulsion changes the electron density, and this change must be compensated by the change in electron density due to the change in external potential. That is, formally one choose the change in the external potential so that,

$$\int \frac{\delta \rho^{\lambda_0}_{n^{\lambda_0},w^{\lambda_0}}(\mathbf{r})}{\delta w(\mathbf{r}')} \left[\frac{dw^{\lambda}(\mathbf{r}')}{d\lambda}\right]_{\lambda=\lambda_0} d\mathbf{r}' = \left[\frac{d\rho^{\mu}_{n^{\lambda_0},w^{\lambda_0}}(\mathbf{r})}{d\mu}\right]_{\mu=\lambda_0} \tag{42}$$

The existence of the constant-density adiabatic connection for ground states is usually assumed without rationalization, and we are unaware of any argument in the literature that goes beyond the assumption that Eq. (42) has a solution. Note also that Eq. (42) is valid only for nondegenerate states, where the linear response function is well defined.

We now provide a stronger and more general justification for the existence of the constant-density adiabatic connection. Suppose the state of interest is $g^{\lambda_0}$-fold degenerate, with eigenstates of $\hat{H}^{\lambda_0}_{w^{\lambda_0}}$ that are degenerate with $\Psi^{\lambda_0}_{n} = \Psi^{\lambda_0}_{n^{\lambda_0},w^{\lambda_0}}$ denoted $\left\{\Psi^{\lambda_0}_{p}\right\}$ and those which are nondegenerate denoted $\left\{\Psi^{\lambda_0}_{k}\right\}$. We now divide the space of potential variations, $\delta w^{\lambda_0}(\mathbf{r})$, into two complementary subspaces. One subspace, $W^{\lambda_0}$, has co-dimension $g^{\lambda_0} - 1$ and corresponds to potential variations, $\delta w(\mathbf{r})$ for which the change in electron density is first order. For $\delta w(\mathbf{r}) \in W^{\lambda_0}$,

$$0 = \left\langle \Psi^{\lambda_0}_{p} \middle| \sum_{i=1}^{N} \delta w(\mathbf{r}_i) \middle| \Psi^{\lambda_0}_{n} \right\rangle \qquad \forall p \text{ with } E^{\lambda_0}_{p,w^{\lambda_0}} = E^{\lambda_0}_{n^{\lambda_0},w^{\lambda_0}} \tag{43}$$

The complementary subspace, $(W^{\lambda_0})'$ has dimension $g-1$ and satisfies the constraints

$$\begin{aligned} 0 &= \left\langle \Psi^{\lambda_0}_{k} \middle| \sum_{i=1}^{N} \delta w(\mathbf{r}_i) \middle| \Psi^{\lambda_0}_{n} \right\rangle \qquad \forall k \text{ with } E^{\lambda_0}_{k,w^{\lambda_0}} \neq E^{\lambda_0}_{n^{\lambda_0},w^{\lambda_0}} \\ 0 &\neq \left\langle \Psi^{\lambda_0}_{p} \middle| \sum_{i=1}^{N} \delta w(\mathbf{r}_i) \middle| \Psi^{\lambda_0}_{n} \right\rangle \qquad \exists p \text{ with } E^{\lambda_0}_{p,w^{\lambda_0}} = E^{\lambda_0}_{n^{\lambda_0},w^{\lambda_0}} \end{aligned} \tag{44}$$

Any external potential can be decomposed into its components in the relevant potential subspaces,

$$w(\mathbf{r}) = w_W(\mathbf{r}) + w_{W'}(\mathbf{r}) \qquad \text{where } w_W(\mathbf{r}) \in W^{\lambda_0} \text{ and } w_{W'}(\mathbf{r}) \in (W^{\lambda_0})' \tag{45}$$

**Note.** *The space of potentials is a Banach space, and not every subspace of a Banach space is complemented. However, every Banach subspace with finite dimension (or, equivalently, finite co-dimension) is complemented, which establishes the validity of the decomposition (45). Functions in the finite-dimensional subspace* $(W^{\lambda_0})'$ *can always be expanded in a basis, but this is not true for the (uncountably infinite dimensional) subspace* $W^{\lambda_0}$*. In particular, each basis function defines a one-dimensional subspace of* $(W^{\lambda_0})'$*. For example, one could choose linearly independent basis functions* $\omega_p(\mathbf{r})$ *that give zero for all but one of Eqs. (44), with the remaining equation,*

$$1 = \left\langle \Psi^{\lambda_0}_{p} \middle| \sum_{i=1}^{N} \omega_p(\mathbf{r}_i) \middle| \Psi^{\lambda_0}_{n} \right\rangle \tag{46}$$

To determine how the density depends on the Hamiltonian (40) we use degenerate perturbation theory. To avoid an $\mathcal{O}(1)$ change in the electron density due to an infinitesimal change in the external potential and interaction strength, we need to ensure that

$$\begin{aligned} 0 &= \left\langle \Psi_p^{\lambda_0} \middle| \left[\frac{\partial \hat{H}^{\mu}_{w^\lambda}}{\partial \lambda}\right]_{\lambda=\mu=\lambda_0} + \left[\frac{\partial \hat{H}^{\mu}_{w^\lambda}}{\partial \mu}\right]_{\lambda=\mu=\lambda_0} \middle| \Psi_n^{\lambda_0} \right\rangle \qquad \left\{ p \,\middle|\, E^{\lambda_0}_{p,w^{\lambda_0}} = E^{\lambda_0}_{n^{\lambda_0},w^{\lambda_0}} \right\} \\ 0 &= \left\langle \Psi_p^{\lambda_0} \middle| \sum_{i=1}^{N} \left[\frac{dw^\lambda(\mathbf{r}_i)}{d\lambda}\right]_{\lambda=\lambda_0} + V_{ee} \middle| \Psi_n^{\lambda_0} \right\rangle \qquad \left\{ p \,\middle|\, E^{\lambda_0}_{p,w^{\lambda_0}} = E^{\lambda_0}_{n^{\lambda_0},w^{\lambda_0}} \right\} \end{aligned} \tag{47}$$

Let $\{\omega_q(\mathbf{r})\}_{q=1}^{g^{\lambda_0}-1} \in (W^{\lambda_0})'$ be a linearly independent basis for the complementary subspace and write

$$\left[\frac{dw^\lambda(\mathbf{r}_i)}{d\lambda}\right]_{\lambda=\lambda_0} = \sum_{q=1}^{g^{\lambda_0}-1} \nu_q \omega_q(\mathbf{r}) \tag{48}$$

Then we need to solve the nonsingular system of $g^{\lambda_0}-1$ linear equations,

$$\sum_{q=1}^{g^{\lambda_0}-1} \left\langle \Psi_p^{\lambda_0} \middle| \sum_{i=1}^{N} \omega_q(\mathbf{r}_i) \middle| \Psi_n^{\lambda_0} \right\rangle \nu_q = -\left\langle \Psi_p^{\lambda_0} \middle| V_{ee} \middle| \Psi_n^{\lambda_0} \right\rangle \qquad \left\{ p \,\middle|\, E^{\lambda_0}_{p,w^{\lambda_0}} = E^{\lambda_0}_{n^{\lambda_0},w^{\lambda_0}} \right\} \tag{49}$$

This determines the part of $\left[\frac{dw^\lambda(\mathbf{r}_i)}{d\lambda}\right]_{\lambda=\lambda_0}$ that lies in the complementary subspace, $(W^{\lambda_0})'$. Note that the change in potential defined in Eq. (48) usually *breaks* the degeneracy. This is important, because the degree of degeneracy, $g^\lambda$, can change repeatedly along the adibatic connection. The only requirement is that one selects a perturbation in $(W^{\lambda_0})'$ such that even after the perturbation, there is a state in the degenerate manifold of states with the desired electron density.

We now need to deduce the portion of $\left[\frac{dw^\lambda(\mathbf{r})}{d\lambda}\right]_{\lambda=\lambda_0}$ that lies in $W^{\lambda_0}$. Perturbations of the potential that lie in $W^{\lambda_0}$ change the density to at most first order, with the change in density given by the expression,

$$\left[\frac{\partial \rho^{\mu}_{n,w^\lambda}(\mathbf{r})}{\partial \lambda}\right]_{\lambda=\mu=\lambda_0} = \sum_{\left\{ k \,\middle|\, E^{\lambda_0}_{k,w^{\lambda_0}} \neq E^{\lambda_0}_{n^{\lambda_0},w^{\lambda_0}} \right\}} \frac{\left\langle \Psi_n^{\lambda_0} \middle| \hat{\rho}(\mathbf{r}) \middle| \Psi_k^{\lambda_0} \right\rangle \left\langle \Psi_k^{\lambda_0} \middle| \sum_{i=1}^{N} \left[\frac{dw^\lambda(\mathbf{r}_i)}{d\lambda}\right]_{\lambda=\lambda_0} \middle| \Psi_n^{\lambda_0} \right\rangle}{E^{\lambda_0}_{n^{\lambda_0},w^{\lambda_0}} - E^{\lambda_0}_{k^{\lambda_0},w^{\lambda_0}}} + c.c. \tag{50}$$

where $\hat{\rho(\mathbf{r})} = \sum_{i=1}^{N} \delta(\mathbf{r}_i - \mathbf{r})$ is the electron-density operator. Eq. (50) can be compared to the expression for the density change induced by a change in the electron-electron repulsion strength,

$$\left[\frac{\partial \rho^{\mu}_{n,w^\lambda}(\mathbf{r})}{\partial \mu}\right]_{\lambda=\mu=\lambda_0} = \sum_{\left\{ k \,\middle|\, E^{\lambda_0}_{k,w^{\lambda_0}} \neq E^{\lambda_0}_{n^{\lambda_0},w^{\lambda_0}} \right\}} \frac{\left\langle \Psi_n^{\lambda_0} \middle| \hat{\rho}(\mathbf{r}) \middle| \Psi_k^{\lambda_0} \right\rangle \left\langle \Psi_k^{\lambda_0} \middle| V_{ee} \middle| \Psi_n^{\lambda_0} \right\rangle}{E^{\lambda_0}_{n^{\lambda_0},w^{\lambda_0}} - E^{\lambda_0}_{k^{\lambda_0},w^{\lambda_0}}} + c.c. \tag{51}$$

These equations effectively expand the change in density using the transition densities,

$$\rho_{kn}(\mathbf{r}) = \left\langle \Psi_n^{\lambda_0} \middle| \hat{\rho}(\mathbf{r}) \middle| \Psi_k^{\lambda_0} \right\rangle + c.c. \tag{52}$$

This is reasonable given that the space of densities has a countable basis. (Note, however that in general the full space of densities would require one to consider *all* the transition densities, not just those linking to the $n^{\text{th}}$ stationary state. The other transition densities appear in second-order perturbation theory.)

The portion of $\left[\frac{dw^\lambda(\mathbf{r})}{d\lambda}\right]_{\lambda=\lambda_0}$ that lies in $W^{\lambda_0}$ is determined by solving the system of linear equations defined by:

$$0 = \left[\frac{\partial \rho^{\mu}_{n,w^\lambda}(\mathbf{r})}{\partial \lambda}\right]_{\lambda=\mu=\lambda_0} - \left[\frac{\partial \rho^{\mu}_{n,w^\lambda}(\mathbf{r})}{\partial \mu}\right]_{\lambda=\mu=\lambda_0} \tag{53}$$

Note that this is a countable system of equations but that the space of potentials, $W^{\lambda_0}$, has uncountable dimension, so it would be very surprising for a solution not to exist.

*Assume* that the transition densities in Eq. (52) are linearly independent. In this case, the linear system is nonsingular and one simply needs to find $\delta w(\mathbf{r}) \in W^{\lambda_0}$ for which

$$\left\langle \Psi_k^{\lambda_0} \middle| \sum_{i=1}^{N} \delta w(\mathbf{r}_i) \middle| \Psi_n^{\lambda_0} \right\rangle = -\left\langle \Psi_k^{\lambda_0} \middle| V_{ee} \middle| \Psi_n^{\lambda_0} \right\rangle \qquad \left\{ k \,\middle|\, E_{k,w^{\lambda_0}}^{\lambda_0} \neq E_{n^{\lambda_0},w^{\lambda_0}}^{\lambda_0} \right\} \tag{54}$$

As this system of linear equations (vastly) underdetermines $\delta w(\mathbf{r})$, one expects solutions and there exists some choice for $\left[\frac{dw^{\lambda}(\mathbf{r}_i)}{d\lambda}\right]_{\lambda=\lambda_0}$ such that the isodensity constraint is retained along the adiabatic connection pathway.

When the transition densities are linearly dependent the system of linear equations is singular. Then Eq. (54) is sufficient (but not necessary) for the existence of the constant-density adiabatic connection. This nominally corresponds to the case where there are multiple choices for $\frac{dw^{\lambda}(\mathbf{r}}{d\lambda})$ that are consistent with the isodensity condition. However, Theorem 7 of reference [12] indicates that external potentials which correspond to the same excited-state electron density are isolated, suggesting that this does not occur.

In summary, we decompose $\frac{dw(\mathbf{r})}{d\lambda}$ into its parts in the complementary subspaces $W^{\lambda_0}$ (defined by Eqs. (43)) and $(W^{\lambda_0})'$ (satisfying Eqs. (44)). The second subspace contains potentials that couple the wavefunction, $\Psi_{n,w}^{\lambda_0}$ to other wavefunctions with the same energy; the change in potential obtained by solving Eqs. (49) ensures that any zeroth-order change in the electron density induced by an infinitesimal change in the electron-electron interaction strength is compensated by an infinitesimal change in external potential, $\delta w'(\mathbf{r}) \in (W^{\lambda_0})'$. The first subspace contains potentials that couple $\Psi_{n,w}^{\lambda_0}$ to other wavefunctions with different energy; the change in potential obtained by solving Eqs. (54) ensures that any first-order change in the electron density induced by an infinitesimal change in the electron-electron interaction strength is compensated by an infinitesimal change in external potential, $\delta w(\mathbf{r}) \in W^{\lambda_0}$. The density variation defined as $\delta w(\mathbf{r}) + \delta w'(\mathbf{r})$ then suffices to maintain constant density along the adiabatic connection pathway.

This justifies the existence of the constant-density adiabatic connection pathway for both ground and excited states, revealing that the presumption of a constant-density adiabatic connection for excited states is no less justified than its ground-state analogue. Note, however, that we assumed that the spectrum of the Hamiltonian was discrete and that the radius of convergence of (degenerate) perturbation theory is nonzero. (The assumption that (degenerate) perturbation theory has nonzero radius of convergence is also essential to the proofs of Theorem 1 and 2.) We also note that (a) there are subtleties related to the solution of an infinite-dimensional system of linear equations and (b) consistent with Eq. (33), we assume that we can integrate $\frac{dw^{\lambda}(\mathbf{r})}{d\lambda}$ along the adiabatic connection path, so that we may define

$$w^{\lambda_0}(\mathbf{r}) = w^1(\mathbf{r}) + \int_1^{\lambda_0} \frac{dw^{\lambda}(\mathbf{r})}{d\lambda} d\lambda. \tag{55}$$

Finally, we mention that Eqs. (54) and the underlying Eq. (53) should not be used for numerical modelling of the adiabatic connection. When there are only a finite number of excited states, these systems are underdetermined, and many unphysical solutions exist. This problem is well known in the optimized effective potential community, and reformulations similar to those employed there could be used here also.

---


[1] E. H. Lieb, Density functionals for coulomb systems, International Journal of Quantum Chemistry **24**, 243 (1983).

[2] W. T. Yang, P. W. Ayers, and Q. Wu, Potential functionals: Dual to density functionals and solution to the upsilon-representability problem, Physical Review Letters **92**, 146404 (2004).

[3] K. A. Dawson and N. H. March, Density Functional Theories Which Are Upper-Bounds to the Hartree-Fock Limit in One Dimension, Physics Letters A **106**, 161 (1984).

[4] I. A. Howard, N. H. March, and P. W. Ayers, Idempotent density matrix derived from a local potential V(r) in terms of HOMO and LUMO properties, Chemical Physics Letters **385**, 231 (2004).

[5] P. W. Ayers, Generalized Christoffel-Darboux formulae and the frontier Kohn-Sham molecular orbitals, Theoretical Chemistry Accounts **110**, 267 (2003).

[6] M. Levy and P. W. Ayers, Kinetic energy from a single Kohn-Sham orbital, Physical Review A **79**, 064504 (2009).

[7] J. Harris and R. O. Jones, The surface energy of a bounded electron gas, J.Phys.F **4**, 1170 (1974).

[8] D. C. Langreth and J. P. Perdew, Exchange-correlation energy ofa metallic surface: Wave-vector analysis, Physical Review B **15**, 2884 (1977).

[9] A. Gorling, Density-functional theory beyond the hohenberg-kohn theorem, Physical Review A **59**, 3359 (1999).

[10] J. Harris, Adiabatic-connection approach to Kohn-Sham theory, Physical Review A **29**, 1648 (1984).
[11] W. Yang, Generalized adiabatic connection in density functional theory, Journal of Chemical Physics **109**, 10107 (1998).
[12] P. W. Ayers and M. Levy, Time-independent (static) density-functional theories for pure excited states: Extensions and unification, Physical Review A **80**, 012508 (2009), 1050-2947.
